# Supplementary material for: Reinforced Imitative Graph Representation Learning for Mobile User Profiling: An Adversarial Training Perspective
Source: arXiv:2101.02634 source file (2021-01-07)
Supplement: Supplementary file 1 [file appendix.tex]

\section{Appendix A}
\subsection{Data Segmentation}
In the experiment, we conduct our experiments on New York and Beijing datasets.
Each dataset is divided into two independent parts: for check-in and taxi data, the prior $90\%$ are the training set, and the remaining $10\%$ are the testing set.
In addition, the dimension of user representation is 200; 
in the spatial knowledge graph ({\it KG}), the dimension of entity ({\it e.g.} POI, POI Category and Locations) and relationship ({\it e.g.}``locate at",``belong to") is 200 respectively.

\subsection{Baselines}
\begin{enumerate}
    \item \textbf{PMF} We use the code \footnote{\url{https://github.com/fuhailin/Probabilistic-Matrix-Factorization}} to implement PMF and utilize the default parameter value in the package to train PMF.
    
    \item \textbf{PoolNet} we adopt ``spotlight'' \footnote{\url{https://github.com/maciejkula/spotlight}} to implement PoolNet.
     We set the learning rate of 0.01 to train PoolNet and other parameters are used default value.
    
    \item \textbf{WaveNet} we utilize ``spotlight'' to implement WaveNet.
    We set the learning rate of 0.01 to train WaveNet and other parameters are used default value.
    
    \item \textbf{LSTMNet} we use ``spotlight'' to implement LSTMNet.
    We set the learning rate of 0.01 to train LSTMNet and other parameters are used default value.
    
    \item \textbf{StructRL} we set the parameters of StructRL based on \cite{wang2019adversarial}. 
    
    \item \textbf{IMUP-r} We use the code \footnote{\url{https://github.com/pwangDM/KDD2020}} to implement IMUP-r. 
    We use the default parameter value to train the model.
   Specially, we set the sampling strategy with reward-based in the model. 
    
    \item \textbf{IMUP-TD} We use the same code as \textbf{IMUP-r} to implement IMUP-TD.
    We use the default parameter value to train the model.
   Specially, we set the sampling strategy with TD-based in the model.

\end{enumerate}

\subsection{Experiment Platform}
All experiments are conducted on Ubuntu 18.04.3 LTS, Intel(R) Core(TM) i9-9920X CPU@ 3.50GHz, with Titan RTX and the memory size is 128G.

\subsection{Parameters of RIRL}

\begin{enumerate}
    \item \textbf{lr$_1$} represents  learning rate of the representation module. 
    \item \textbf{lr$_2$} represents the learning rate of the imitation module.
    \item \textbf{ld} represents the weight of $r_d$ that is the reciprocal of the distance between the real and predicted visit POI.
    \item \textbf{lc} represents the weight of $r_c$ that is the similarity between the real and predicted POI category.
    \item \textbf{lp} represents the weight of $r_p$ that whether the predicted POI is the real one.
    \item \textbf{memory\_capacity} represents the capacity of the replay buffer in the imitation module (DQN).
    \item \textbf{batch\_size} represents the sampling batch size in the imitation module (DQN).
    \item \textbf{epsilon} represents the probability that the model picks up a possible POI randomly.
    \item \textbf{gamma} represents the value of gamma of the Bellman Equation in the imitation module (DQN). 
    \item \textbf{time\_window} represents the size of the time window that is used to calculate the reward balance.
    \item \textbf{target\_replace\_iter} represents in the imitation module (DQN), the target network update their parameters are target\_replace\_iter slower than the evaluation network.
    \item \textbf{sampling\_strategy} represents the sampling strategy in the imitation module.
    ``r'' is reward-based sampling strategy. 
    ``td'' is TD-based sampling strategy.
    \item \textbf{cross\_validation}.
    This parameter is used to control our conducting experiment.
    There are two values for cross\_validation:
    0 represents the overall performance experiment;
    1 represents the robustness check experiment.
    
\end{enumerate}

\subsection{Experimental Setting}

\subsubsection{Overall Experiments}

\begin{enumerate}

    \item New York Dataset
    \begin{enumerate}
        \item RIRL-r.
        lr$_1$ : 0.001; 
        lr$_2$ : 0.0001;
        ld : 0.2;
        lc : 0.6;
        lp : 0.2;
        memory\_capacity : 128;
        batch\_size : 32;
        epsilon : 0.97;
        gamma : 0.94;
        time\_window : 5;
        target\_replace\_iter : 5;
        sampling\_strategy : ``r''
        cross\_validation : 0;
        
        \item RIRL-TD.
        lr$_1$ : 0.001; 
        lr$_2$ : 0.0001;
        ld : 0.44;
        lc : 0.33;
        lp : 0.23;
        memory\_capacity : 20;
        batch\_size : 10;
        epsilon : 0.98;
        gamma : 0.85;
        time\_window : 5;
        target\_replace\_iter : 5;
        sampling\_strategy : ``td''
        cross\_validation : 0;
        
    \end{enumerate}

    \item Beijing Dataset
    \begin{enumerate}
        \item RIRL-r.
        
        lr$_1$ : 0.001; 
        lr$_2$ : 0.001;
        ld : 0.45;
        lc : 0.3;
        lp : 0.25;
        memory\_capacity : 64;
        batch\_size : 25;
        epsilon : 0.92;
        gamma : 0.99;
        time\_window : 5;
        target\_replace\_iter : 5;
        sampling\_strategy : ``r''.
        cross\_validation : 0;
        
        \item RIRL-TD.
        
         lr$_1$ : 0.001; 
        lr$_2$ : 0.01;
        ld : 0.31;
        lc : 0.08;
        lp : 0.61;
        memory\_capacity : 64;
        batch\_size : 15;
        epsilon : 0.95;
        gamma : 0.75;
        time\_window : 5;
        target\_replace\_iter : 5;
        sampling\_strategy : ``td''.
        cross\_validation : 0;
        
    \end{enumerate}
    
\end{enumerate}

\subsection{Robustness Check}
\begin{enumerate}
    \item New York Dataset
    \begin{enumerate}
        \item RIRL-r
        
        lr$_1$ : 0.001; 
        lr$_2$ : 0.0001;
        ld : 0.53;
        lc : 0.12;
        lp : 0.35;
        memory\_capacity : 64;
        batch\_size : 25;
        epsilon : 0.94;
        gamma : 0.8;
        time\_window : 5;
        target\_replace\_iter : 5;
        sampling\_strategy : ``r''
        cross\_validation : 1;
        
        \item RIRL-TD
        
        lr$_1$ : 0.001; 
        lr$_2$ : 0.0001;
        ld : 0.57;
        lc : 0.07;
        lp : 0.36;
        memory\_capacity : 128;
        batch\_size : 40;
        epsilon : 0.98;
        gamma : 0.88;
        time\_window : 5;
        target\_replace\_iter : 5;
        sampling\_strategy : ``TD''
        cross\_validation : 1;
        
    \end{enumerate}
    
    \item Beijing Dataset
    \begin{enumerate}
        \item RIRL-r
        lr$_1$ : 0.001; 
        lr$_2$ : 0.0001;
        ld : 0.3;
        lc : 0.4;
        lp : 0.3;
        memory\_capacity : 64;
        batch\_size : 25;
        epsilon : 0.9;
        gamma : 0.85;
        time\_window : 5;
        target\_replace\_iter : 5;
        sampling\_strategy : ``r''
        cross\_validation : 1;
        
        \item RIRL-TD
        
         lr$_1$ : 0.001; 
        lr$_2$ : 0.0001;
        ld : 0.2;
        lc : 0.7;
        lp : 0.1;
        memory\_capacity : 64;
        batch\_size : 32;
        epsilon : 0.93;
        gamma : 0.9;
        time\_window : 5;
        target\_replace\_iter : 5;
        sampling\_strategy : ``TD'';
        cross\_validation : 1;
    \end{enumerate}
\end{enumerate}

\subsection{The guideline for AAAI Code}

We recommend you to install anaconda as your basic python library, here our code is running on python 3.7.4, then you can use this code according to the following steps.

\begin{enumerate}
    \item Download our code to your local machine:
    
    \item
    Unzip the zip file.
    If you use windows or mac, you can double click the zip file. Otherwise, you can use unzip command to unzip the code.
    
    \item We recommend you to create one specific environment for this code, if you do not care about this issue, you can skip to step 5.
    The command is ``conda create -n AAAItest python=3.7.4''
    
    \item Activate the python environment.
    The command is ``conda activate AAAItest''
    
    \item Install all required python packages, we have provided the requirements file, so you can use following command.
    ``pip install -r requirements.txt''
    
    \item Run this code.
    ``python main.py''
    
    \item If you want to change the experiment parameters, you can use following commands:
    
    \begin{enumerate}
        \item Beijing Dataset
        
        ``python main.py --priority\_mode='r' --city='bj' --model\_name='dqn' --reward\_mode='r1' --ll=0.3 --lc=0.3 --lp=0.4 --memory\_capacity=20 --batch\_size=6 --lr=0.001 --epsilon=0.9 --gamma=0.9 --target\_replace\_iter=5 --data\_batch\_size=1024 --user\_path='./newdata/bj/s\_user.pkl' --poi\_dist\_mat\_path='./newdata/bj/poi\_dist\_Mat.pkl' --cat\_sim\_mat\_path='./newdata/bj/cat\_sim\_mat.pkl' --s\_KG\_path='./newdata/bj/s\_KG.pkl' --poi\_cat\_dict\_path='./newdata/bj/POI\_cat\_dict.pkl' --poi\_loc\_dict\_path='./newdata/bj/POI\_loc\_dict.pkl' --poi\_list\_train\_path='./newdata/bj/POI\_list\_train.pkl' --user\_list\_train\_path='./newdata/bj/user\_list\_train.pkl' --temporal\_train\_path='./newdata/bj/Temporal\_train.pkl' --poi\_list\_test\_path='./newdata/bj/POI\_list\_test.pkl' --user\_list\_test\_path='./newdata/bj/user\_list\_test.pkl' --temporal\_test\_path='./newdata/bj/Temporal\_test.pkl' --cross\_validation=0''
        
        \item NewYork Dataset
        
        ``python main.py --priority\_mode='r' --city='nyc' --model\_name='dqn' --reward\_mode='r1' --ll=0.3 --lc=0.3 --lp=0.4 --memory\_capacity=20 --batch\_size=6 --lr=0.001 --epsilon=0.9 --gamma=0.9 --target\_replace\_iter=5 --data\_batch\_size=1024 --user\_path='./newdata/nyc/s\_user.pkl' --poi\_dist\_mat\_path='./newdata/nyc/poi\_dist\_Mat.pkl' --cat\_sim\_mat\_path='./newdata/nyc/cat\_sim\_mat.pkl' --s\_KG\_path='./newdata/nyc/s\_KG.pkl' --poi\_cat\_dict\_path='./newdata/nyc/POI\_cat\_dict.pkl' --poi\_loc\_dict\_path='./newdata/nyc/POI\_loc\_dict.pkl' --poi\_list\_train\_path='./newdata/nyc/POI\_list\_train.pkl' --user\_list\_train\_path='./newdata/nyc/user\_list\_train.pkl' --temporal\_train\_path='./newdata/nyc/Temporal\_train.pkl' --poi\_list\_test\_path='./newdata/nyc/POI\_list\_test.pkl' --user\_list\_test\_path='./newdata/nyc/user\_list\_test.pkl' --temporal\_test\_path='./newdata/nyc/Temporal\_test.pkl' --cross\_validation=0''
    \end{enumerate}
    
   If you want to reproduce the experimental results, please use the parameter value in the section of \textbf{Experiment Setting}.
    Owing to the randomness of reinforcement learning, the experimental results have a little fluctuation, but from the overall perspective, the experimental results are stable.
    
\end{enumerate}
